# Supplementary material for: Pressure-induced trans-proximate correlation in La$_4$Ni$_3$O$_{10}$ and possible routes to enhance its superconductivity
Source: arXiv:2505.13442 source file (2025-10-27)
Supplement: Supplementary file 1 [file Supplementary.pdf]

# Supplemental materials: Emergence of cross-layer composite spins in $La_4Ni_3O_{10}$ under pressure and possible routes to enhance its superconductivity

Ruoshi Jiang, Zhiyu Fan, Bartomeu Monserrat, and Wei Ku

## I. CRYSTAL STRUCTURE OF $LA_4NI_3O_{10}$ UNDER PRESSURE

Following Ref. [S1], the crystal structure of $La_4Ni_3O_{10}$ at ambient pressure corresponds to monoclinic space group $P2_1/a$ with lattice parameters $a = 5.4164$ Å, $b = 5.4675$ Å, $c = 14.2279$ Å, and $\beta = 100.752°$ . The crystal structure of $La_4Ni_3O_{10}$ at 44.3 GPa corresponds to tetragonal space group $I4/mmm$ with lattice parameters $a = 3.6606$ Å, $b = 3.6606$Å, and $c = 26.277$Å. The two local structures are depicted in Fig. S1, with the main difference between the two structures being the straightening of the Ni-O-Ni-O-Ni bond within the trilayer structure in the high pressure regime.

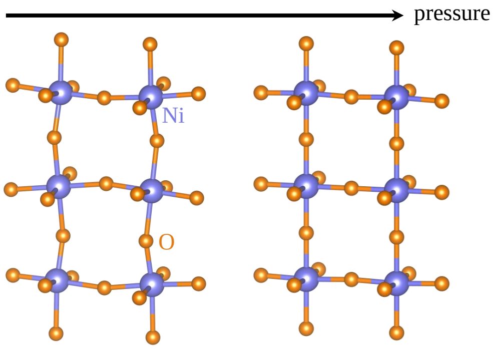


FIG. S1. Comparison of the low-pressure and high-pressure crystal structures of $La_4Ni_3O_{10}$.

## II. COMPUTATIONAL DETAILS OF THE DENSITY FUNCTIONAL THEORY CALCULATIONS

The most relevant energy window of trilayer $La_4Ni_3O_{10}$ corresponds to 15 eV about the Fermi energy. We characterize the associated electronic structure using the spin polarized LDA+$U$ [S2, S3] approximation to density functional theory (DFT) [S4, S5] as implemented within the linearized augmented plane wave method [S6] in the WIEN2K package [S7]. Following a previous study [S8], we use a typical value of $U - J = 6$ eV for Ni $d$-orbitals, and we confirm that our qualitative results are insensitive to this parameter up to at least a 1 eV variation.

## III. COMPUTING THE BAND STRUCTURE IN THE NON-COLLINEAR CURIE-PARAMAGNETIC PHASE

Transition metal oxides with open electron $d$ shells are subject to strong intra-atomic Coulomb repulsion. The standard local density approximation (LDA) of DFT does not capture these interactions, resulting in unphysically large charge fluctuations. Intra-atomic Coulomb interactions can be incorporated using the LDA+$U$ method, which pushes most electrons away from the Fermi energy and leads to more accurate charge densities. However, it is often necessary to use spin-polarized DFT+$U$ calculations to accomplish this, forcing the system to exhibit long-range magnetic order.

This spin-polarized approach becomes problematic when the system has fluctuating local moments without long-range magnetic order, such as in a quantum Curie-paramagnetic phase of strongly correlated metals or geometrically frustrated magnets. For example, spin-polarized calculations may produce an incorrect charge carrier distribution when the relevant energy scale is higher than that of inter-atomic magnetic correlations and the resulting behaviour is insensitive to a particular long-range magnetic order. In these situations, it is beneficial to have access to the band structure through the one-body spectral function in a simulated Curie-paramagnetic phase, in which inter-atomic magnetic correlations are negligible, such that the impact of the (artificial) magnetic order is removed.

This one-body spectral function can be obtained using standard DFT by averaging the 'unfolded' one-particle spectral function [S9] of an ensemble of large supercells, each containing an instance of disordered *non-collinear* spin orientations on each

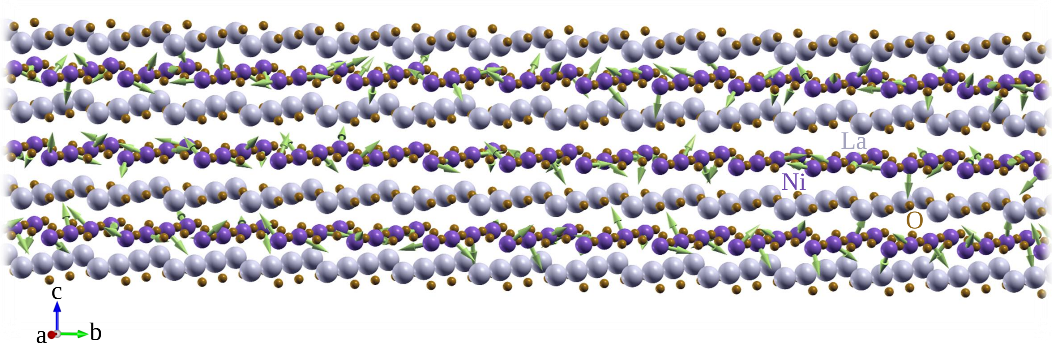


FIG. S2. Illustration of *unordered non-collinear* Curie paramagnetic configurations of high-pressure phase with spin directions of each magnetic atom Ni denoted by the green arrows.

transition metal ion. The smallness of the magnetic correlations in each supercell can be checked by calculating the corresponding magnetic correlation function $\chi(r) = \sum_i \mathbf{S}_{i+r} \cdot \mathbf{S}_i$. Figure S2 gives an example of such a supercell used in this study. In addition, it helps to reduce the artificial periodicity of the supercells if they are chosen in various sizes, shapes and orientations [S10].

It is possible to reduce the computational cost of the above procedure by constructing a SU(2)-symmetric interacting Hamiltonian using, for example, the method described in the Sec. V below. While this is not physically necessary, the reduced Hilbert space dramatically reduces the computational expense, enabling the use of larger supercells that better resemble the magnetically disordered systems.

## IV. ATOMIC WANNIER ORBITALS AS A BASIS FOR $H^{(\mathbf{Hartree})}$

The Hartree-scale physics is best described using atomically local orbitals as a basis. We therefore construct a complete set of atomic-like Ni $d$-, O $p$-, and La $d$- and $f$-Wannier orbitals [S11–S13] without down-folding to the one-body low-energy subspace. These symmetry-respecting Wannier orbitals form a nearly complete atomically local basis that is nearly configuration independent, making them ideal for the ensemble averaging to construct the one-particle spectral function discussed in Sec. III above.

## V. EXTRACTION OF THE INTERACTING $H^{(\mathbf{Hartree})}$ FROM DFT CALCULATIONS

In transition metal oxides, the open-shell $d$-electrons exhibit suppressed charge fluctuations due to the large intra-atomic Coulomb repulsion $U$. This can be described using a generic SU(2) *symmetric* interacting Hamiltonian $H^{(\text{Hartree})}$:

$$\begin{aligned} H^{(\text{Hartree})} = & \sum_{i,i',m,m',\nu} t_{ii'mm'} c^\dagger_{im\nu} c_{i'm'\nu} \\ & + \frac{1}{2} \sum_{i,m,m',m'',m''',\nu,\nu'} U_{mm''m'm'''} c^\dagger_{im\nu} c^\dagger_{im''\nu'} c_{im'''\nu'} c_{im'\nu} \\ & - \sum_{i,m,m',\nu} V^{\text{HF0}}_{mm'} c^\dagger_{im\nu} c_{im'\nu}, \end{aligned} \tag{S1}$$

where $t$ denotes the one-body hopping strength, $U$ the intra-atomic two-body Coulomb interaction of Ni, and $c^\dagger_{im\nu}$ the creation operators of orbitals $m$ and spin $\nu$ at lattice site $i$. Note that, for convenience, $t$ also includes the contribution from the spin-averaged Hartree-Fock mean field, $V^{\text{HF0}}$, so the latter is subtracted in the last line of Eq. S1.

To parametrize the Hamiltonian in Eq. S1 using DFT, it is often necessary to use spin-polarized DFT+$U$ as explained in Sec. III above. We fix the parameters in Eq. S1 by requiring it to reproduce the DFT+$U$ band structure under *various* magnetic structures with a single set of parameters [S10, S12, S14], via the same self-consistent Hartree-Fock approximation as employed in DFT+$U$ [S15]. Specifically, the corresponding density matrix $\rho_{i\nu\nu'}$ must be identical in both cases when represented in the same set of Wannier orbitals. One can thus take $\rho_{i\nu\nu'}$ directly from the self-consistent LDA+$U$ solution in the Wannier basis. The procedure can be simplified by assuming that the structure of $U_{mm''m'm'''}$ follows the Slater integral fixed by two parameters $U_{\text{eff}}$ and $J_{\text{eff}}$ [S3, S16]. Combining $\rho_{i\nu\nu'}$ and $U_{mm''m'm'''}$, the effective Hartree-Fock potential $V^{\text{HF}}$ can then obtained. Furthermore,

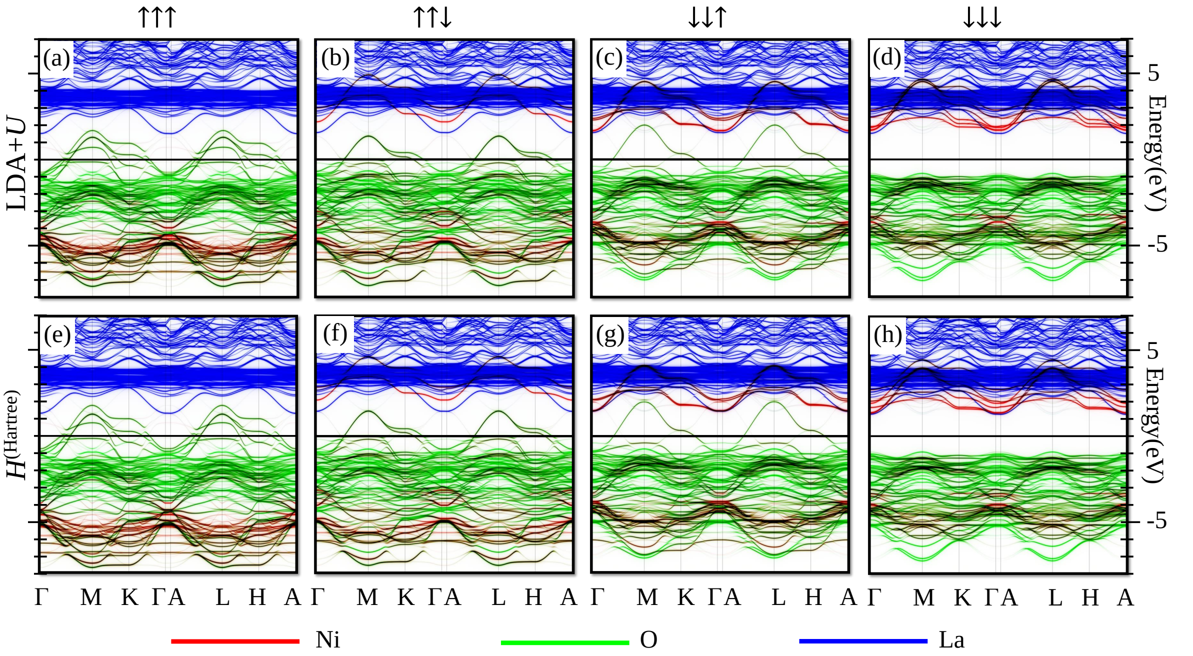


FIG. S3. Quality verification of $H^{(\text{Hartree})}$ for the low-pressure phase, by reproducing the LDA+$U$ band structures under (a)↑↑↑, (b)↑↑↓, (c)↓↓↑ and (d)↓↓↓ magnetic structure, with its self-consistent Hartree-Fock results in (e)-(h) using a fixed set of parameter.

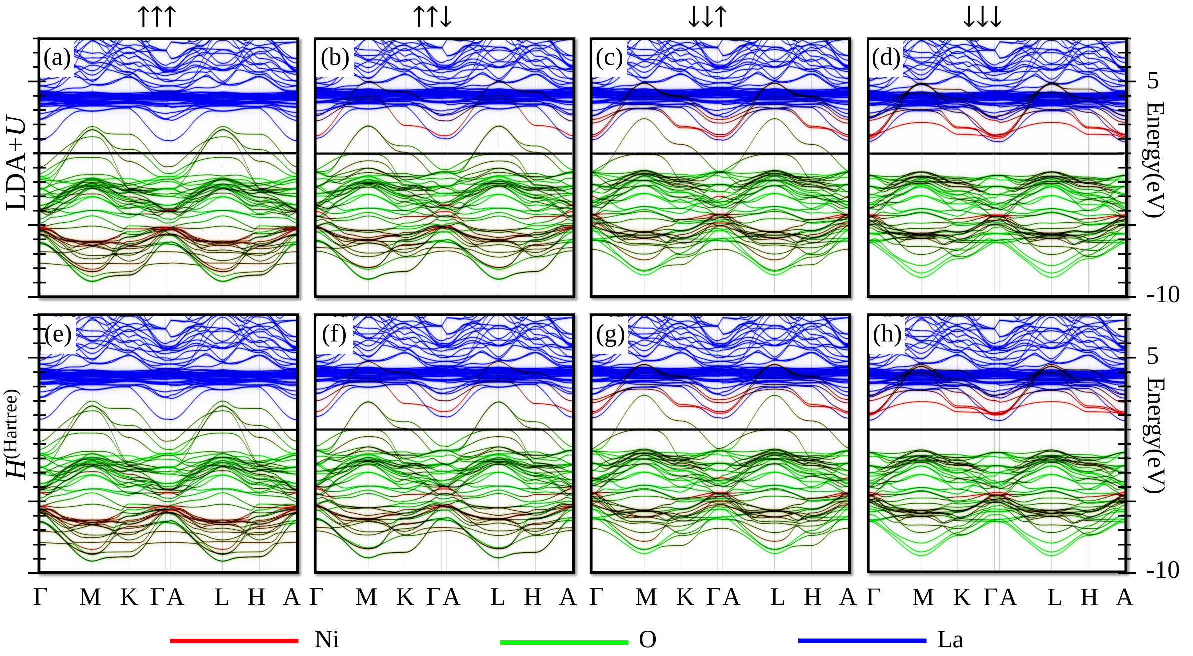


FIG. S4. Same as Fig. S3, but for the high-pressure phase.

we find that the $t$ parameters are quite insensitive to the magnetic structure, so one typically can just take the spin-average of that obtained from the Wannier functions.

Figure S3 compares the LDA+$U$ band structures of the low-pressure phase with those obtained from the Hartree-Fock approximation applied to our extracted Hamiltonian $H^{(\text{Hartree})}$ under various common magnetic configurations: ↑↑↑, ↑↑↓, ↓↓↑, and ↓↓↓. A single $H^{(\text{Hartree})}$ with a fixed set of parameters is able to reproduce all the LDA+$U$ band structures. Figure S4 shows the corresponding results for the high-pressure phase, and the corresponding (distinct) single parameter set for $H^{(\text{Hartree})}$ also leads to good agreement with the LDA+$U$ results. This comparison therefore confirms the quality of the parametrized $H^{(\text{Hartree})}$ for both phases.

Even though we have established the quality of $H^{(\mathrm{Hartree})}$ by comparing its approximate (Hartree-Fock) solutions against the corresponding DFT+$U$ results, we can further use $H^{(\mathrm{Hartree})}$ beyond this approximate treatment, and we can also explore $H^{(\mathrm{Hartree})}$ in phases that are not magnetically ordered. As we demonstrate in this work, the SU(2) symmetric interacting Hamiltonian of Eq. S1 encodes emergent low-energy physics to explain the microscopic properties of $La_4Ni_3O_{10}$.

## VI. LEADING PARAMETERS OF $H^{(\mathrm{Hartree})}$

Using the strategy discussed above in Sec. V, we find ($U_{\mathrm{eff}}$, $J_{\mathrm{eff}}$) $\sim$ (6.26, 1.2) eV for the middle Ni in the trilayer, and (5.85, 1.16) eV for the upper and lower Ni in the low-pressure phase; and ($U_{\mathrm{eff}}$, $J_{\mathrm{eff}}$) $\sim$ (6.12, 1.18) eV for the middle Ni and (6.12, 1.14) eV for the upper and lower Ni in the high-pressure phase. The key hopping parameters are provided in Tab. 1 of the main text, and the full set of $t_{ii'mm'}$ parameters are available upon request.

## VII. OBTAINING THE LOW-ENERGY EFFECTIVE HAMILTONIAN VIA A NUMERICAL CANONICAL TRANSFORMATION

A low-energy effective theory can capture the key physics of a quantum system within a well-defined energy scale. Conceptually, it can be rigorously constructed by integrating out the high-energy states in a path integral formulation. Equivalently, it can also be derived by decoupling the low-energy states of interest from the remaining high-energy states. Specifically, consider the second quantized basis $\{a_i, a_i^\dagger\}$ spanning the one-body space indexed by $i$. If there exists a unitary transformation $\hat{U}[\{a_i, a_i^\dagger\}]$ given by [S17, S18]:

$$\tilde{a}_i^\dagger = \hat{U}^\dagger a_i^\dagger \hat{U}, \tag{S2}$$

that transforms the Hamiltonian into a 'block diagonal' form $\tilde{H}$, then in the new 'many-body dressed' representation $\tilde{a}_i$, the low-energy subspace is decoupled from the high-energy subspace:

$$\tilde{H}[\{\tilde{a}_i, \tilde{a}_i^\dagger\}] \equiv H[\{a_i, a_i^\dagger\}] = H[\{\hat{U}\tilde{a}_i\hat{U}^\dagger, \hat{U}\tilde{a}_i^\dagger\hat{U}^\dagger\}] = \hat{U}H[\{\tilde{a}_i, \tilde{a}_i^\dagger\}]\hat{U}^\dagger. \tag{S3}$$

The block diagonalization can be performed numerically by applying successive unitary transformations until the unwanted off-diagonal block, $P^{(\mathrm{L})}HP^{(\mathrm{H})}$, is suppressed below some tolerance, with $P^{(\mathrm{L})}$ and $P^{(\mathrm{H})} \equiv 1 - P^{(\mathrm{L})}$ being the projection operators for the low- and high-energy subspaces. Additionally, if the 'rotational angle' of each transformation is small, each unitary transformation can be performed using the low order terms in the expansion:

$$\tilde{H} = e^A H e^{-A} = H + [A, H] + \frac{1}{2!}[A, [A, H]] + \cdots, \tag{S4}$$

using a 'small' anti-Hermitian operator $A$ that generates each unitary transformation $\hat{U} = e^A$. Specifically, for each term $C$ in $P^{(\mathrm{L})}HP^{(\mathrm{H})}$, $A$ then includes a contribution $\alpha(C - C^\dagger)$ with the sign (and magnitude) of $\alpha$ chosen to reduce the resulting unwanted block. In some cases, special care should be taken when choosing $\alpha$ for each contribution of $A$ to ensure the proper symmetry of the representation.

Upon reaching a satisfactory level of accuracy with negligible $P^{(\mathrm{L})}\tilde{H}P^{(\mathrm{H})}$, the low-energy effective Hamiltonian can then be taken from the low-energy sector of $\tilde{H}$,

$$H' = P^{(\mathrm{L})}\tilde{H}P^{(\mathrm{L})}. \tag{S5}$$

We also note that the above procedure can be repeated to obtain even lower-energy scale Hamiltonians by identifying another set of leading high-energy states to 'integrate out' and construct the corresponding projection operators.

In practice, we implement the above procedure algebraically by developing a suite of C++ programs designed to numerically manipulate second-quantized operators. This includes evaluating commutators and enforcing normal ordering, as required by the methodology. The results derived from this computational framework are cross-validated against those obtained from the analytical approach outlined in Section VIII, with both methods demonstrating full consistency.

A significant reduction in computational cost can be achieved by restricting the Hilbert space of interest *a priori*. As an important example, most physical Hamiltonians conserve the particle number $N$, and so do the corresponding $A$ and $\hat{U}$ operators. One can therefore apply a projection operator $P_N$ of the subspace with fixed particle number $N$ to $H \to P_N H P_N$ at any stage of the procedure. $P_N$ can be practically implemented as $P_N = P_{\leq N}\, P_{\geq N}$, where $P_{\geq N}$ is the $N$-body representation of the identity operator in second-quantized notation that ensures at least $N$ particles are present in the system, and $P_{\leq N}$ corresponds to the

truncation of all terms involving more than $N$-body terms at any stage of the computation. In many cases, we find that applying it to $P^{(L)} \to P_N P^{(L)}$, if possible, is the easiest and most efficient strategy.

In this study, three sets of high-energy states are integrated out at different energy scales. At the Hartree scale, the high-energy states are the states containing charged Ni ions with double occupied configurations. The corresponding projection operator is:

$$P^{(\mathrm{L})} = (1 - X_\uparrow^\dagger X_\downarrow^\dagger X_\downarrow X_\uparrow)^{(\mathrm{u})}(1 - Z_\uparrow^\dagger Z_\downarrow^\dagger Z_\downarrow Z_\uparrow)^{(\mathrm{u})}(1 - X_\uparrow^\dagger X_\downarrow^\dagger X_\downarrow X_\uparrow)^{(\mathrm{m})}(1 - Z_\uparrow^\dagger Z_\downarrow^\dagger Z_\downarrow Z_\uparrow)^{(\mathrm{m})}(1 - X_\uparrow^\dagger X_\downarrow^\dagger X_\downarrow X_\uparrow)^{(\mathrm{l})}(1 - Z_\uparrow^\dagger Z_\downarrow^\dagger Z_\downarrow Z_\uparrow)^{(\mathrm{l})}, \quad (\mathrm{S6})$$

where $X_\uparrow^\dagger$ and $Z_\uparrow^\dagger$ denote creation of a spin-up electron in the $d_{x^2-y^2}$ and $d_{3z^2-r^2}$ orbitals, respectively, of Ni in the upper (u), middle (m), and lower (l) layers of the Ni-O-Ni-O-Ni trilayer. Further absorbing the particle number projection $P_N$ for $N = 10$ to $P^{(L)}$ gives

$$\begin{aligned} P_N =& p_\uparrow^{1\dagger} p_\downarrow^{1\dagger} p_\downarrow^1 p_\uparrow^1 p_\uparrow^{2\dagger} p_\downarrow^{2\dagger} p_\downarrow^2 p_\uparrow^2 \\ & (X_\uparrow^\dagger X_\uparrow + X_\downarrow^\dagger X_\downarrow)^{(\mathrm{u})} (Z_\uparrow^\dagger Z_\uparrow + Z_\downarrow^\dagger Z_\downarrow)^{(\mathrm{u})} (X_\uparrow^\dagger X_\uparrow + X_\downarrow^\dagger X_\downarrow)^{(\mathrm{m})} (Z_\uparrow^\dagger Z_\uparrow + Z_\downarrow^\dagger Z_\downarrow)^{(\mathrm{m})} (X_\uparrow^\dagger X_\uparrow + X_\downarrow^\dagger X_\downarrow)^{(\mathrm{l})} (Z_\uparrow^\dagger Z_\uparrow + Z_\downarrow^\dagger Z_\downarrow)^{(\mathrm{l})}, \end{aligned} \quad (\mathrm{S7})$$

where $p_\uparrow^{1\dagger}$ and $p_\uparrow^{2\dagger}$ denote creation of a spin-up electron in the $p_z$ orbital of the apical $O_1^{(\mathrm{m})}$ and $O_2^{(\mathrm{m})}$ between the Ni atoms.

As discussed in the main text, $P_N P^{(L)}$ above corresponds to a low-energy subspace with double occupation of $p_z$ orbitals and single occupation for the remaining orbitals. Applying the above procedure then gives $H^{(\mathrm{eV})} = P_N P^{(\mathrm{L})} \tilde{H} P^{(\mathrm{L})}$ in Eq. (1) of the main text.

At the eV scale, the Hund's coupling $\tilde{J}_\mathrm{H}$ dominates in the low-pressure phase, and the high-energy states are those containing a spin singlet $W^\dagger |0\rangle$ among the $d_{3z^2-r^2}$ and $d_{x^2-y^2}$ orbitals within the same Ni ion, denoted by the singlet creation operator:

$$W^\dagger = \frac{1}{\sqrt{2}}(X_\uparrow^\dagger Z_\downarrow^\dagger - X_\downarrow^\dagger Z_\uparrow^\dagger). \quad (\mathrm{S8})$$

Applying the above procedure with the projection operator:

$$P^{(\mathrm{L})} = (1 - W^\dagger W)^{(\mathrm{u})}(1 - W^\dagger W)^{(\mathrm{m})}(1 - W^\dagger W)^{(\mathrm{l})}, \quad (\mathrm{S9})$$

results in $H^{(\text{sub-eV})}$, as written in Eq. (2) of the main text, with a spin-1 effective $Ni^{2+}$ ionic spin $\mathbf{S}_\mathrm{eff}$.

In contrast, for the high-pressure phase dominated by inter-layer anti-ferromagnetic super-exchange $J_{ZZ}$, the low-energy states are those containing a spin doublet among the $d_{x^2-y^2}$ orbitals of the Ni ions across the Ni-O-Ni-O-Ni trilayer. Expressed via the creation operator of the remaining *inter*-layer doublet:

$$V_\uparrow^\dagger = \frac{1}{\sqrt{6}}[Z_\uparrow^{\dagger(\mathrm{u})} Z_\uparrow^{\dagger(\mathrm{m})} Z_\downarrow^{\dagger(\mathrm{l})} - 2 Z_\uparrow^{\dagger(\mathrm{u})} Z_\downarrow^{\dagger(\mathrm{m})} Z_\uparrow^{\dagger(\mathrm{l})} + Z_\downarrow^{\dagger(\mathrm{u})} Z_\uparrow^{\dagger(\mathrm{m})} Z_\uparrow^{\dagger(\mathrm{l})}], \quad (\mathrm{S10})$$

$$V_\downarrow^\dagger = \frac{1}{\sqrt{6}}[Z_\downarrow^{\dagger(\mathrm{u})} Z_\downarrow^{\dagger(\mathrm{m})} Z_\uparrow^{\dagger(\mathrm{l})} - 2 Z_\downarrow^{\dagger(\mathrm{u})} Z_\uparrow^{\dagger(\mathrm{m})} Z_\downarrow^{\dagger(\mathrm{l})} + Z_\uparrow^{\dagger(\mathrm{u})} Z_\downarrow^{\dagger(\mathrm{m})} Z_\downarrow^{\dagger(\mathrm{l})}], \quad (\mathrm{S11})$$

the projection operator for the low-energy subspace is:

$$P^{(\mathrm{L})} = V_\uparrow^\dagger V_\uparrow + V_\downarrow^\dagger V_\downarrow. \quad (\mathrm{S12})$$

The above procedure then gives $H^{(\text{sub-eV})}$ in Eq. (3) of the main text, with a fractionalized spin-1/2 effective ionic spin $\mathbf{S}_\mathrm{eff}$ for each $Ni^{2+}$ ion, and drives the formation of a cross-layer trimer composite $\frac{1}{2}$-spin.

## VIII. ALTERNATIVE DERIVATION OF EFFECTIVE HAMILTONIANS

Section VII describes the derivation of low-energy effective Hamiltonians using second quantized operators and their non-commuting algebra. Instead, in this section we demonstrate the process of deriving a low-energy effective Hamiltonian using an alternative implementation of the above general idea within the first quantization formalism via the vector space of the many-body states.

In trilayer $La_4Ni_3O_{10}$, the local Ni-O-Ni-O-Ni unit hosts 960 many-body states within its 8 orbitals and 10-electron configuration. These states span a subspace with distinct $z$-components of the total spin ($S_z$), which remain decoupled from other many-body states due to symmetry constraints. The general strategy is:

1. *Identify the low- and high-energy subspace.*

   We construct the full many-body matrix representation of the Hamiltonian (in normal-ordered form), which enables the identification of the low-energy subspace with single occupation and of the high-energy subspace with double occupation on Ni orbitals. This separation is driven by the strong Coulomb interactions energetically isolating double-occupied configurations to high-energy states.

2. *Decouple the high-energy subspace from the remaining low-energy space.*

   We decouple the high-energy subspace from the remaining low-energy space via the numerical unitary transformation. The low-energy sector of the Hamiltonian matrix naturally corresponds to the low-energy effective Hamiltonian $H^{(\mathrm{eV})}$ with the single occupied configurations, while the high-energy states containing double occupied configurations in Ni orbtials.

The resulting subspace containing 64 many-body states explicitly captures the dominant spin-orbital correlations and interactions with single electron occupations on Ni. The matrix elements of this low-energy block can then be systematically mapped to a second-quantized representation of $H^{(\mathrm{eV})}$ as in Eq. (1) of the main text, where the effective degrees of freedom emerge from the entanglement structure of the original Hilbert space.

(a)

| | | | | | | | | | | | | | | |
|---|---|---|---|---|---|---|---|---|---|---|---|---|---|---|
| -0.66 | 0 | 0 | 0 | 0 | 0 | 0 | 0 | 0.18 | 0 | 0 | 0 | 0.18 | 0 | 0 |
| 0 | -0.48 | 0 | 0 | 0 | 0 | 0 | 0.18 | 0 | 0 | 0 | 0 | 0 | 0 | 0 |
| 0 | 0 | -0.48 | 0 | 0 | 0 | 0 | 0 | 0 | 0 | 0 | 0.18 | 0 | 0 | 0 |
| 0 | 0 | 0 | 0.35 | 0 | -0.32 | -0.32 | 0 | 0 | 0 | 0 | 0 | 0 | 0 | 0 |
| 0 | 0 | 0 | 0 | -0.01 | -0.32 | -0.32 | 0 | 0 | 0.18 | 0 | 0 | 0 | 0.18 | 0 |
| 0 | 0 | 0 | -0.32 | -0.32 | 0.17 | 0 | 0.18 | 0 | 0 | 0 | 0 | 0 | 0 | 0 |
| 0 | 0 | 0 | -0.32 | -0.32 | 0 | 0.17 | 0 | 0 | 0 | 0 | 0.18 | 0 | 0 | 0 |
| 0 | 0.18 | 0 | 0 | 0 | 0.18 | 0 | -0.02 | 0 | -0.32 | -0.32 | 0 | 0 | 0 | 0 |
| 0.18 | 0 | 0 | 0 | 0 | 0 | 0 | 0 | 0.16 | -0.32 | -0.32 | 0 | 0 | 0 | 0 |
| 0 | 0 | 0 | 0 | 0.18 | 0 | 0 | -0.32 | -0.32 | 0.16 | 0 | 0 | 0 | 0 | 0 |
| 0 | 0 | 0 | 0 | 0 | 0 | 0 | -0.32 | -0.32 | 0 | 0.34 | 0 | 0 | 0 | 0 |
| 0 | 0 | 0.18 | 0 | 0 | 0 | 0.18 | 0 | 0 | 0 | 0 | -0.02 | 0 | -0.32 | -0.32 |
| 0.18 | 0 | 0 | 0 | 0 | 0 | 0 | 0 | 0 | 0 | 0 | 0 | 0.16 | -0.32 | -0.32 |
| 0 | 0 | 0 | 0 | 0.18 | 0 | 0 | 0 | 0 | 0 | 0 | -0.32 | -0.32 | 0.16 | 0 |
| 0 | 0 | 0 | 0 | 0 | 0 | 0 | 0 | 0 | 0 | 0 | -0.32 | -0.32 | 0 | 0.34 |

Change → Basis

(b)

| | | | | | | | | | | | | | | |
|---|---|---|---|---|---|---|---|---|---|---|---|---|---|---|
| -0.66 | 0 | 0 | 0 | 0 | 0 | 0 | 0.09 | 0.13 | 0.00 | 0.09 | 0.09 | 0.13 | 0 | 0.09 |
| 0 | -0.48 | 0 | 0 | 0 | 0 | 0 | 0.09 | -0.13 | 0.00 | 0.09 | 0 | 0 | 0 | 0 |
| 0 | 0 | -0.48 | 0 | 0 | 0 | 0 | 0 | 0 | 0 | 0 | 0.09 | -0.13 | 0 | 0.09 |
| 0 | 0 | 0 | -0.48 | -0.13 | 0 | 0 | 0.09 | -0.06 | 0.06 | 0 | 0.09 | -0.06 | 0.06 | 0 |
| 0 | 0 | 0 | -0.13 | 0.17 | 0 | -0.13 | 0.06 | 0 | 0.09 | -0.06 | 0.06 | 0 | 0.09 | -0.06 |
| 0 | 0 | 0 | 0 | 0 | 0.17 | 0 | 0.06 | -0.09 | 0 | 0.06 | -0.06 | 0.09 | 0.00 | -0.06 |
| 0 | 0 | 0 | 0 | -0.13 | 0 | 0.82 | 0 | 0.06 | 0.06 | -0.09 | 0 | 0.06 | 0.06 | -0.09 |
| 0.09 | 0.09 | 0 | 0.09 | 0.06 | 0.06 | 0 | -0.48 | 0.06 | -0.06 | -0.09 | 0 | 0 | 0 | 0 |
| 0.13 | -0.13 | 0 | -0.06 | 0 | -0.09 | 0.06 | 0.06 | 0.07 | 0.01 | 0.06 | 0 | 0 | 0 | 0 |
| 0 | 0 | 0 | 0.06 | 0.09 | 0 | 0.06 | -0.06 | 0.01 | 0.25 | 0.06 | 0 | 0 | 0 | 0 |
| 0.09 | 0.09 | 0 | 0 | -0.06 | 0.06 | -0.09 | -0.09 | 0.06 | 0.06 | 0.80 | 0 | 0 | 0 | 0 |
| 0.09 | 0 | 0.09 | 0.09 | 0.06 | -0.06 | 0 | 0 | 0 | 0 | 0 | -0.48 | 0.06 | -0.06 | -0.09 |
| 0.13 | 0 | -0.13 | -0.06 | 0 | 0.09 | 0.06 | 0 | 0 | 0 | 0 | 0.06 | 0.07 | 0.01 | 0.06 |
| 0 | 0 | 0 | 0.06 | 0.09 | 0 | 0.06 | 0 | 0 | 0 | 0 | -0.06 | 0.01 | 0.25 | 0.06 |
| 0.09 | 0 | 0.09 | 0 | -0.06 | -0.06 | -0.09 | 0 | 0 | 0 | 0 | -0.09 | 0.06 | 0.06 | 0.80 |

↓ Resequence

(c)

| | | | | | | | | | | | | | | |
|---|---|---|---|---|---|---|---|---|---|---|---|---|---|---|
| -0.66 | 0 | 0 | 0 | 0.09 | 0.09 | 0.13 | 0.13 | 0 | 0 | 0 | 0 | 0.09 | 0.09 | 0 |
| 0 | -0.48 | 0 | 0 | 0.09 | 0 | -0.13 | 0 | 0 | 0 | 0 | 0 | 0.09 | 0 | 0 |
| 0 | 0 | -0.48 | 0 | 0 | 0.09 | 0 | -0.13 | 0 | 0 | 0 | 0 | 0 | 0.09 | 0 |
| 0 | 0 | 0 | -0.48 | 0.09 | 0.09 | -0.06 | -0.06 | -0.13 | 0 | 0.06 | 0.06 | 0 | 0 | 0 |
| 0.09 | 0.09 | 0 | 0.09 | -0.48 | 0 | 0.06 | 0 | 0.06 | 0.06 | -0.06 | 0 | -0.09 | 0 | 0 |
| 0.09 | 0 | 0.09 | 0.09 | 0 | -0.48 | 0 | 0.06 | 0.06 | -0.06 | 0 | -0.06 | 0 | -0.09 | 0 |
| 0.13 | -0.13 | 0 | -0.06 | 0.06 | 0 | 0.07 | 0 | 0 | -0.09 | 0.01 | 0 | 0.06 | 0 | 0.06 |
| 0.13 | 0 | -0.13 | -0.06 | 0 | 0.06 | 0 | 0.07 | 0 | 0.09 | 0 | 0.01 | 0 | 0.06 | 0.06 |
| 0 | 0 | 0 | -0.13 | 0.06 | 0.06 | 0 | 0 | 0.17 | 0 | 0.09 | 0.09 | -0.06 | -0.06 | -0.13 |
| 0 | 0 | 0 | 0 | 0.06 | -0.06 | -0.09 | 0.09 | 0 | 0.17 | 0 | 0 | 0.06 | -0.06 | 0 |
| 0 | 0 | 0 | 0.06 | -0.06 | 0 | 0.01 | 0 | 0.09 | 0 | 0.25 | 0 | 0.06 | 0 | 0.06 |
| 0 | 0 | 0 | 0.06 | 0 | -0.06 | 0 | 0.01 | 0.09 | 0 | 0 | 0.25 | 0 | 0.06 | 0.06 |
| 0.09 | 0.09 | 0 | 0 | -0.09 | 0 | 0.06 | 0 | -0.06 | 0.06 | 0.06 | 0 | 0.80 | 0 | -0.09 |
| 0.09 | 0 | 0.09 | 0 | 0 | -0.09 | 0 | 0.06 | -0.06 | -0.06 | 0 | 0.06 | 0 | 0.80 | -0.09 |
| 0 | 0 | 0 | 0 | 0 | 0 | 0.06 | 0.06 | -0.13 | 0 | 0.06 | 0.06 | -0.09 | -0.09 | 0.82 |

← Block diagonal

(d)

| | | | | | | | | | | | | | | |
|---|---|---|---|---|---|---|---|---|---|---|---|---|---|---|
| -0.72 | 0.02 | 0.02 | 0.02 | 0.08 | 0.08 | | | | | | | | | |
| 0.02 | -0.52 | 0.00 | -0.01 | 0.11 | 0.00 | | | | | | | | | |
| 0.02 | 0.00 | -0.52 | -0.01 | 0.00 | 0.11 | | | | | | | | | |
| 0.02 | -0.01 | -0.01 | -0.53 | 0.11 | 0.11 | | | | | | | | | |
| 0.08 | 0.11 | 0.00 | 0.11 | -0.51 | 0.00 | | | | | | | | | |
| 0.08 | 0.00 | 0.11 | 0.11 | 0.00 | -0.51 | | | | | | | | | |
| | | | | | | 0.13 | 0.03 | 0.02 | -0.08 | 0.00 | -0.01 | 0.05 | 0.01 | 0.06 |
| | | | | | | 0.03 | 0.13 | 0.02 | 0.08 | -0.01 | 0.00 | 0.01 | 0.05 | 0.06 |
| | | | | | | 0.02 | 0.02 | 0.20 | 0.00 | 0.07 | 0.07 | -0.07 | -0.07 | -0.13 |
| | | | | | | -0.08 | 0.08 | 0.00 | 0.18 | -0.01 | 0.01 | 0.06 | -0.06 | 0.00 |
| | | | | | | 0.00 | -0.01 | 0.07 | -0.01 | 0.26 | 0.01 | 0.07 | 0.00 | 0.06 |
| | | | | | | -0.01 | 0.00 | 0.07 | 0.01 | 0.01 | 0.26 | 0.00 | 0.07 | 0.06 |
| | | | | | | 0.05 | 0.01 | -0.07 | 0.06 | 0.07 | 0.00 | 0.82 | 0.00 | -0.09 |
| | | | | | | 0.01 | 0.05 | -0.07 | -0.06 | 0.00 | 0.07 | 0.00 | 0.82 | -0.09 |
| | | | | | | 0.06 | 0.06 | -0.13 | 0.00 | 0.06 | 0.06 | -0.09 | -0.09 | 0.82 |

FIG. S5. Examples of deriving $H^{(\mathrm{sub\text{-}eV})}$ from $H^{(\mathrm{eV})}$ (in unit of eV) in the subspace with $Sz = 1$-component of total spin. (a) Identify the leading physics ($\tilde{J}_{\mathrm{H}}$) and the corresponding off-diagonal terms in green. (b) Zero out these terms via unitary transformation to identify the low-energy subspace (with spin-1 Ni ions). (c) Re-sequence for an easier visualization. (d) Decouple the low-energy sector (in blue) from the rest via block diagonalization. The resulting upper left block gives the low-energy effective $H^{(\mathrm{sub\text{-}eV})}$. Empty cells correspond to those with identical zero values (up to machine accuracy), while '0.00' represents values smaller than 0.01 in size.

The same procedure can be repeated for the derivation of even lower-energy Hamiltonians $H^{(\mathrm{sub\text{-}eV})}$ starting from the effective $H^{(\mathrm{eV})}$ Hamiltonian, and an example of doing this for the low-pressure phase is illustrated in Fig. S5. Figure S6(a) lists the many-body states that span a subspace with a $Sz = 1$-component of the total spin. For the low-pressure phase, the corresponding many-body matrix for the sequence of the many-body states is shown in Fig. S5(a), where the renormalized ferromagnetic Hund's coupling $\tilde{J}_{\mathrm{H}} \sim 0.6\,\mathrm{eV}$ dominates within individual Ni ions. Since $\tilde{J}_{\mathrm{H}}$ introduces off-diagonal terms in the current many-body representation, we perform a sequence of symmetry-preserving unitary transformations on $H^{(\mathrm{eV})}$, which systematically rotate the basis to one where $\tilde{J}_{\mathrm{H}}$ becomes approximately diagonal in Fig. S5(b). The new basis now explicitly shows a 3+1 eigen-structure with 1) low-energy states: spin-1 configurations favored by Hund's coupling and 2) high-energy states: spin-0 configurations on Ni ions suppressed by Hund's coupling. In the transformed basis, the Hamiltonian matrix naturally partitions into high-energy and low-energy blocks with an onsite energy difference of about 0.6 eV.

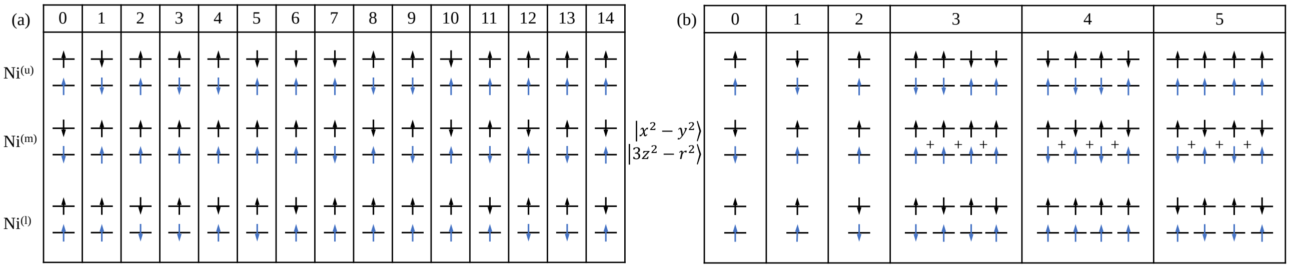


FIG. S6. (a)Illustration of local many-body states of Ni-O-Ni-O-Ni trilayer component in the subspace with $Sz = 1$ for the eV scale. (b)The low-energy many-body states for the blue region in Fig. S5 (c).

The low-energy block now encodes the subspace of spin-1 Ni states coupled via residual interactions. Figure. S6(b) lists the low-energy many-body states for the blue region in Fig. S5(c). Projecting the low-energy block into this spin-1 subspace yields $H^{(\text{sub-eV})}$, as shown in Fig. S5(d), which now incorporates the renormalized inter-site spin exchange of effective $Ni^{2+}$ ionic spin-1 $\mathbf{S}_{\text{eff}}$ and emergent biquadratic terms due to virtual fluctuations into high-energy states:

$$\begin{aligned} H_{\text{LP}}^{(\text{sub-eV})} &= J^{(\text{ml})}\,(\mathbf{S}_{\text{eff}}^{(\text{m})}\cdot\mathbf{S}_{\text{eff}}^{(\text{u})}+\mathbf{S}_{\text{eff}}^{(\text{m})}\cdot\mathbf{S}_{\text{eff}}^{(\text{l})})+J^{(\text{ul})}\,\mathbf{S}_{\text{eff}}^{(\text{u})}\cdot\mathbf{S}_{\text{eff}}^{(\text{l})} \\ &+K^{(\text{ul})}\Big[(\mathbf{S}_{\text{eff}}^{(\text{m})}\cdot\mathbf{S}_{\text{eff}}^{(\text{u})})(\mathbf{S}_{\text{eff}}^{(\text{m})}\cdot\mathbf{S}_{\text{eff}}^{(\text{l})})+(\mathbf{S}_{\text{eff}}^{(\text{m})}\cdot\mathbf{S}_{\text{eff}}^{(\text{l})})(\mathbf{S}_{\text{eff}}^{(\text{m})}\cdot\mathbf{S}_{\text{eff}}^{(\text{u})})\Big] \\ &+K^{(\text{ll})}\,\Big[(\mathbf{S}_{\text{eff}}^{(\text{m})}\cdot\mathbf{S}_{\text{eff}}^{(\text{u})})(\mathbf{S}_{\text{eff}}^{(\text{m})}\cdot\mathbf{S}_{\text{eff}}^{(\text{u})})+(\mathbf{S}_{\text{eff}}^{(\text{m})}\cdot\mathbf{S}_{\text{eff}}^{(\text{l})})(\mathbf{S}_{\text{eff}}^{(\text{m})}\cdot\mathbf{S}_{\text{eff}}^{(\text{l})})\Big], \end{aligned} \tag{S13}$$

By contrast, for the high-pressure phase, the dominant inter-layer anti-ferromagnetic super-exchange $J_{ZZ} \sim 0.7\,\text{eV}$ dictates a strong correlation between $\mathbf{S}_Z$ across the trilayer. Applying a numerical canonical transformation to $H^{(\text{eV})}$, perfomed by diagonalizing the $J_{ZZ}$ terms, reveals a well separated 2+2+4 eigen-structure with 1) low-energy states: spin-1/2 configurations $\frac{1}{\sqrt{6}}\,|\uparrow\uparrow\downarrow\rangle - \frac{2}{\sqrt{6}}\,|\uparrow\downarrow\uparrow\rangle + \frac{1}{\sqrt{6}}\,|\downarrow\uparrow\uparrow\rangle$ and 2) high-energy states: spin-1/2 configurations $\frac{1}{\sqrt{2}}\,|\uparrow\uparrow\downarrow\rangle - \frac{1}{\sqrt{2}}\,|\downarrow\uparrow\uparrow\rangle$ and spin-3/2 configurations $\frac{1}{\sqrt{3}}\,|\uparrow\uparrow\downarrow\rangle + \frac{1}{\sqrt{3}}\,|\uparrow\downarrow\uparrow\rangle + \frac{1}{\sqrt{3}}\,|\downarrow\uparrow\uparrow\rangle$ and $|\uparrow\uparrow\uparrow\rangle$ ($S_z > 0$). In the transformed basis, the Hamiltonian matrix naturally partitions into high-energy and low-energy blocks. The low-energy block now corresponds to a cross-layer trimer configuration, which emerges as a composite $\frac{1}{2}$-spin, $\mathbf{S}^{(\text{t})}$, coupled via residual interactions to $\mathbf{S}_{\text{eff}}$. Projecting the low-energy block into this spin-$\frac{1}{2}$ subspace yields $H^{(\text{sub-eV})}$, which now incorporates the renormalized inter-site spin exchange of an effective fractionalized spin-1/2 $\mathbf{S}_{\text{eff}}$ for each $Ni^{2+}$ ion and emergent biquadratic terms due to virtual fluctuations into high-energy states:

$$\begin{aligned} H_{\text{HP}}^{(\text{sub-eV})} &= J^{(\text{mt})}\,\mathbf{S}_{\text{eff}}^{(\text{m})}\cdot\mathbf{S}^{(\text{t})}+J^{(\text{lt})}\,(\mathbf{S}_{\text{eff}}^{(\text{l})}\cdot\mathbf{S}^{(\text{t})}+\mathbf{S}_{\text{eff}}^{(\text{u})}\cdot\mathbf{S}^{(\text{t})}) \\ &+J^{(\text{ul})}\,\mathbf{S}_{\text{eff}}^{(\text{u})}\cdot\mathbf{S}_{\text{eff}}^{(\text{l})}+J^{(\text{ml})}\,(\mathbf{S}_{\text{eff}}^{(\text{m})}\cdot\mathbf{S}_{\text{eff}}^{(\text{u})}+\mathbf{S}_{\text{eff}}^{(\text{m})}\cdot\mathbf{S}_{\text{eff}}^{(\text{l})}) \\ &+K^{(\text{lt})}\Big[(\mathbf{S}_{\text{eff}}^{(\text{m})}\cdot\mathbf{S}_{\text{eff}}^{(\text{u})})(\mathbf{S}_{\text{eff}}^{(\text{l})}\cdot\mathbf{S}^{(\text{t})})+(\mathbf{S}_{\text{eff}}^{(\text{m})}\cdot\mathbf{S}_{\text{eff}}^{(\text{l})})(\mathbf{S}_{\text{eff}}^{(\text{u})}\cdot\mathbf{S}^{(\text{t})})\Big] \\ &+K^{(\text{mt})}\,(\mathbf{S}_{\text{eff}}^{(\text{u})}\cdot\mathbf{S}_{\text{eff}}^{(\text{l})})(\mathbf{S}_{\text{eff}}^{(\text{m})}\cdot\mathbf{S}^{(\text{t})}). \end{aligned} \tag{S14}$$

The detailed parameters governing the sub-eV Hamiltonians are summarized in Tab. S1, and the dominant couplings with magnitudes larger than 0.05 eV are discussed in the main text.

TABLE S1. *The emergence of cross-layer trimer composite spin and the necessity of reducing layer symmtry.* Magnetic coupling strengths in emerged $H^{(\text{sub-eV})}$ are given in unit of eV for the low-pressure and high-pressure phases, derived from $H^{(\text{eV})}$ Hamiltonian with parameters $\tilde{J}_{\text{H}}^{(\text{m})}$, $\tilde{J}_{\text{H}}^{(\text{l})}$ and $J_{ZZ}$.

| | | | | | | |
|---|---|---|---|---|---|---|
| low-pressure | $J^{(\text{ml})}$ | $J^{(\text{ul})}$ | $K^{(\text{ul})}$ | $K^{(\text{ll})}$ | | |
| | **0.11** | −0.02 | 0.01 | 0.02 | | |
| high-pressure | $J^{(\text{lt})}$ | $J^{(\text{mt})}$ | $J^{(\text{ml})}$ | $J^{(\text{ul})}$ | $K^{(\text{lt})}$ | $K^{(\text{mt})}$ |
| | **−0.28** | **0.13** | 0.01 | 0.03 | **0.15** | **−0.09** |

## IX. PARAMETERS IN DERIVING $H^{(\text{eV})}$ FROM $H^{(\text{Hartree})}$

In deriving the local $H^{(\text{eV})}$ from $H^{(\text{Hartree})}$, only a few effective parameters are needed, most of which can be directly obtained from $H^{(\text{Hartree})}$. The kinetic energy $t_{pZ}^{\perp(\text{mm})}$ is $\sim 1.4\,\text{eV}$ and $\sim 2.0\,\text{eV}$, and $t_{pZ}^{\perp(\text{ll})}$ is $\sim 1.4\,\text{eV}$ and $\sim 1.8\,\text{eV}$, for the low-pressure and

high-pressure phases, respectively. The $|d^8p^6d^8\rangle$ to $|d^9p^5d^8\rangle$ charge transfer energy $E_{\rm CT}$ is $\sim 3$ eV. The Coulomb interaction $U_d$ and Hund's coupling $J_{\rm H}$ among Ni-$d$ orbitals are $\sim 6$ eV and $\sim 0.8$ eV, respectively. Note that due to nearly full occupation of O-orbitals, the LDA+$U$ calculation is insensitive to the value of the intra-atomic Coulomb repulsion $U_p$ of the O-orbitals. $U_p$ is therefore absorbed as a local site energy of O orbitals in $H^{(\rm Hartree)}$, and later estimated to be $\sim 4$ eV following the literature [S19]. We checked that our qualitative conclusions are insensitive to variations of 1 eV in $U_p$.

## X. RAPID GROWTH OF $J_{ZZ}$ UPON INCREASING $t^{\perp}_{pZ}$ THROUGH APPLIED PRESSURE

Microscopically, the qualitative change of local physics shown in this work results from the enhancement of $J_{ZZ}$ at the eV scale due to strengthened $t^{\perp}_{pZ}$ at high pressure. Figure S7 shows that this enhancement is rather rapid due to the high-order nature of its emergence (in the perturbative regime it is proportional to $t^{\perp 4}_{pZ}$). This trend should be further enhanced upon the inclusion of additional fluctuations from the itinerant carriers to the spin in the $d_{x^2-y^2}$ orbital, as it can only weaken the effectiveness of $J_{\rm H}$ and in turn further strengthen the high-pressure phase. The observed first-order-like transition, associated with the switching of leading physics from $\tilde{J}_{\rm H}$ to $J_{ZZ}$ at the eV scale, is therefore inescapable (requires no fine-tuning.)

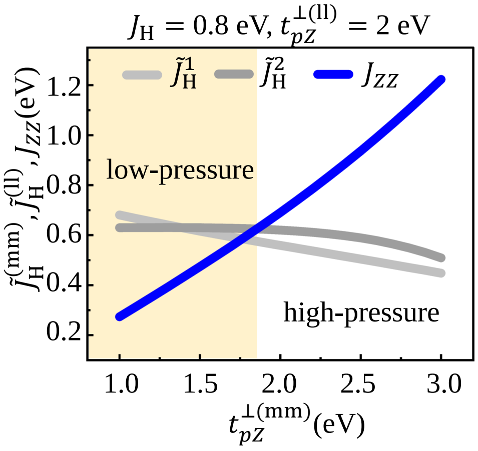


FIG. S7. Rapid growth of inter-layer super-exchange $J_{ZZ}$ at eV-scale due to enhanced $t^{\perp(\rm mm)}_{pZ}$ under higher pressure. In contrast, the intra-atomic Hund's coupling $J_{\rm H}$ is weakly screened. Distinct from the low-pressure phase, the inter-layer super-exchange dominates in the high-pressure phase, leading to fractionalization of the $\rm Ni^{2+}$ ionic spin at sub-eV scale. Note that inclusion of additional fluctuation from the itinerant carriers to the spin in $d_{x^2-y^2}$ orbital will weaken the effectiveness of $J_{\rm H}$ and in turn further strength the high-pressure phase.

## XI. COMPETITION BETWEEN THE HUND'S COUPLING $\tilde{J}_{\rm H}$ AND SUPEREXCHANGE $J_{ZZ}$

As illustrated in Fig. S8, the competition between the renormalized Hund's coupling $\tilde{J}_{\rm H}$ and the inter-layer superexchange $J_{ZZ}$ in determining the low-energy dynamics manifests in the eigenvalue spectrum of $H^{(\rm eV)}$, which evolves systematically with the ratio $J_{ZZ}/\tilde{J}_{\rm H}$. In the limit where $\tilde{J}_{\rm H} \gg J_{ZZ}$ (left), the local intra-atomic spin-$\frac{1}{2}$ pairs on individual Ni ions exhibit a characteristic triplet-singlet splitting, reflecting the dominance of ferromagnetic alignment within atomic orbitals. In contrast, in the limit where $J_{ZZ} \gg \tilde{J}_{\rm H}$ (right), strong oxygen-mediated inter-layer hopping $t^{\perp}_{pZ}$ drives the three inter-atomic spin-$\frac{1}{2}$ states to split into distinct configurations: two doublets and one quartet. The stark contrast between these eV-scale interaction regimes directly underpins the bifurcation between the low- and high-pressure phases of their low-energy physics at the sub-eV scale. This energy-scale separation enables the emergence of composite spin states in the system, offering the natural explanation of the observed weakened superconductivity in trilayer nickelates.

## XII. EFFECTIVE SUB-EV HAMILTONIAN WITH O VACANCY

Starting from the Hartree-scale Hamiltonian, we introduce an O vacancy by neglecting the hopping parameters $t_{pZ}$ between the Ni in the upper and middle layer and the O in the middle layer. Following the many-body downfolding procedure introduced in Secs. VII and VIII above, we derive the sub-eV effective Hamiltonian by projecting out the high-energy states. The resulting

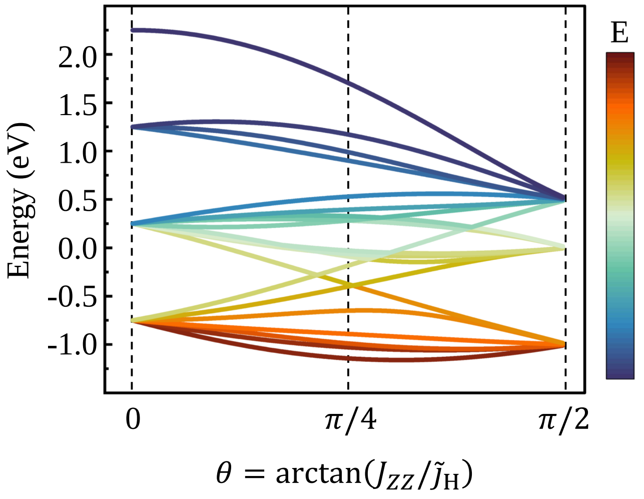


FIG. S8. Competing effect on low-energy dynamics between the Hund's coupling $\tilde{J}_{\mathrm{H}}$ and superexchange $J_{ZZ}$. Notice that the 27+27+9+1 energy splitting for left side and the 16+16+32 energy splitting for the right side within the 64 many-body states.

low-energy physics contains a stand-alone spin-1 $Ni^{2+}$ ion in the upper layer, and fractionalized spin-$\frac{1}{2}$ $Ni^{2+}$ ions in the middle and lower layers that mirrors those in the bilayer nickelates [S8]:

$$H^{(\text{sub-eV})} = J^{(\text{ml})}\, \mathbf{S}_{\text{eff}}^{(\text{m})} \cdot \mathbf{S}_{\text{eff}}^{(\text{l})}, \tag{S15}$$

with $J^{(\text{ml})} \sim 0.13\,\text{eV}$ in the low-pressure phase and $J^{(\text{ml})} \sim 0.08\,\text{eV}$ in the high-pressure phase. The nearly uncoupled spin-$\frac{1}{2}$ $\text{Ni}^{(\text{m})}$ and $\text{Ni}^{(\text{l})}$ ions in the middle and lower layers would recover the efficient spin-fluctuations that facilitate kinetic processes of itinerant carriers and in turn stiffen the superconducting phase.

[S1] J. Li, C.-Q. Chen, C. Huang, Y. Han, M. Huo, X. Huang, P. Ma, Z. Qiu, J. Chen, X. Hu, L. Chen, T. Xie, B. Shen, H. Sun, D.-X. Yao, and M. Wang, Structural transition, electric transport, and electronic structures in the compressed trilayer nickelate $La_4Ni_3O_{10}$, Science China Physics, Mechanics & Astronomy **67** (2024).
[S2] V. I. Anisimov, I. V. Solovyev, M. A. Korotin, M. T. Czyżyk, and G. A. Sawatzky, Density-functional theory and NiO photoemission spectra, Phys. Rev. B **48**, 16929 (1993).
[S3] A. I. Liechtenstein, V. I. Anisimov, and J. Zaanen, Density-functional theory and strong interactions: Orbital ordering in mott-hubbard insulators, Phys. Rev. B **52**, R5467 (1995).
[S4] P. Hohenberg and W. Kohn, Inhomogeneous electron gas, Phys. Rev. **136**, B864 (1964).
[S5] W. Kohn and L. J. Sham, Self-consistent equations including exchange and correlation effects, Phys. Rev. **140**, A1133 (1965).
[S6] D. J. Singh, *Planewaves, Pseudopotentials and the LAPW Method* (Springer New York, NY, New York, 2006).
[S7] P. Blaha, K. Schwarz, P. Sorantin, and S. Trickey, Full-potential, linearized augmented plane wave programs for crystalline systems, Computer Physics Communications **59**, 399 (1990).
[S8] R. Jiang, J. Hou, Z. Fan, Z.-J. Lang, and W. Ku, Pressure driven fractionalization of ionic spins results in cupratelike high-$T_c$ superconductivity in $La_3Ni_2O_7$, Phys. Rev. Lett. **132**, 126503 (2024).
[S9] W. Ku, T. Berlijn, and C.-C. Lee, Unfolding first-principles band structures, Phys. Rev. Lett. **104**, 216401 (2010).
[S10] R. Jiang, Z.-J. Lang, T. Berlijn, and W. Ku, Variation of carrier density in semimetals via short-range correlation: A case study with nickelate $NdNiO_2$, Phys. Rev. B **108**, 155126 (2023).
[S11] W. Ku, H. Rosner, W. E. Pickett, and R. T. Scalettar, Insulating ferromagnetism in $La_4Ba_2Cu_2O_{10}$: An ab initio wannier function analysis, Phys. Rev. Lett. **89**, 167204 (2002).
[S12] W.-G. Yin, D. Volja, and W. Ku, Orbital ordering in $LaMnO_3$: Electron-electron versus electron-lattice interactions, Phys. Rev. Lett. **96**, 116405 (2006).
[S13] N. Marzari and D. Vanderbilt, Maximally localized generalized wannier functions for composite energy bands, Phys. Rev. B **56**, 12847 (1997).
[S14] Z.-J. Lang, R. Jiang, and W. Ku, Strongly correlated doped hole carriers in the superconducting nickelates: Their location, local many-body state, and low-energy effective hamiltonian, Phys. Rev. B **103**, L180502 (2021).
[S15] V. I. Anisimov, F. Aryasetiawan, and A. I. Lichtenstein, First-principles calculations of the electronic structure and spectra of strongly correlated systems: the LDA + $U$ method, Journal of Physics: Condensed Matter **9**, 767 (1997).
[S16] J. Slater, *Quantum Theory of Molecules and Solids* (Mcgram-Hill, New York, 1974).

[S17] K. A. Chao, J. Spalek, and A. M. Oles, Kinetic exchange interaction in a narrow s-band, Journal of Physics C: Solid State Physics **10**, L271 (1977).
[S18] S. White, Numerical canonical transformation approach to quantum many-body problems, The Journal of Chemical Physics **117** (2002).
[S19] M. Ogata and H. Fukuyama, The t–J model for the oxide high-$T_c$ superconductors, Reports on Progress in Physics **71**, 036501 (2008).
